# Supplementary material for: Demonstration of Safe Electromagnetic Radiation Emitted by 5G Active Antenna Systems
Source: arXiv:2406.07910 source file (2024-06-12)
Supplement: Supplementary file 1 [file appendix.tex]

There are two established measures for EMF measurements:
\begin{itemize}
	\item Electric flux density in W/m²
	\item Electric field strength in V/m
\end{itemize}

Both measures are based on power measurements (in dBm). By applying the antenna
factor (in dB/m) and/or the antenna aperture (in m²), power measurements can be
converted into either electric flux density or electric field strength.

Several metrics have been defined for the measurement of EMF such as electric field strength, magnetic field strength, specific absorption ratio and power density.

EMF can be measured by \textit{active} or \textit{passive} scanners. In active scanners, the measurement device has to make connection with the gNB and hence can decode the payload data apart from broadcast channels to measure the EMF. While in the passive scanners the measurement device uses the content of the braodcast channels to assess the EMF. Now, we will briefly discuss the three widely used methods to measure EMF which are also used by the EMF measurement instrument manufacturers. 

\begin{enumerate}
	\item \textbf{Frequency selective EMF measurement[REF]}: In this type of measurement pure power spectrum is measured within the configured frequency band without the identificartion of the carriers/emitters. This measured power is further converted to electric field strength (V/m). This can be done with a simple spectrum analyzer and the antenna factor file[REF]. This method is simple and no decoding of the broadcast channel (and extrapolation) is required. 
	
	\item \textbf{Code selective measurement[REF]}: In this type of measurement the power is computed from the SSBs and converted to electric field strength (V/m). It identify, decodes carriers and beams and then determine precise signal power levels which are converted to electric field strength (V/m). Using this method, different emitters can be distinguished and their emissions can be categorized such as per operator, per cell-site, per sector and per SSB beam. This method is more complex than frequency selective as decoding of the SSBs, extrapolation and compensation of beam gain/offset is required[REF]. However, from the operator point of view, code-selective method is more preferred since the EMF data is obtained per-operator. 
	
	\item \textbf{Broadband measurement[REF]}: In this type of measurement, the power is computed by summing the power of all the signals whose frequency fall under the span of the broadband probe. Gives the total radiation received by a human as observed at the time of measurement. This type of measurement accounts for all types of radiations coming from cellular, WiFi, Bluetooth etc. Nonetheless, this is the cumulative radiation experienced by the human body and used as a reference for overall levels in the environment. 
\end{enumerate}
